# Supplementary material for: Training and re-training liquid crystal elastomer metamaterials for pluripotent functionality
Source: arXiv:2502.17238 source file (2025-02-24)
Supplement: Supplementary file 1 [file SI_retrainable_lces.pdf]

# **Supporting Information for**

## **Training and re-training liquid crystal elastomer metamaterials for pluripotent functionality**

Savannah D. Gowen<sup>a,1</sup>, Elina Ghimire<sup>b</sup>, Charlie A. Lindberg<sup>b</sup>, Ingrid S. Appen<sup>b</sup>, Stuart J. Rowan<sup>b,c</sup>, and Sidney R. Nagel<sup>a</sup>

<sup>a</sup>Department of Physics and The James Franck and Enrico Fermi Institutes, University of Chicago, Chicago, IL 60637, USA; <sup>b</sup>Pritzker School of Molecular Engineering, University of Chicago, Chicago, IL 60637, USA; <sup>c</sup>Department of Chemistry, University of Chicago, Chicago, IL 60637, USA

<sup>1</sup>Corresponding author: Savannah D. Gowen  
Email: savannah.gowen@mat.ethz.ch

### **This PDF file includes:**

Supporting text  
1. Disordered Array Geometry  
2. Training and Temperature  
Instrumentation  
Synthesis schemes  
Figures S1 to S5  
SI References

## Supporting Information Text

**Disordered Array Geometry-** Metamaterial structures are derived from simulated jammed particle packings in which the center of a particle is replaced by a node and particle contacts are replaced by struts. The networks shown have between 30-60 nodes with connectivity between 3-4. Fig.S3 shows the geometries used in these experiments.

**Training and Temperature-** Temperature is used to “speed up” the aging process during the training by enabling the material to adapt more quickly. A set of initial experiments were conducted in which the disordered arrays were compressed in 3hr increments at 50C. The Poisson's ratio,  $\nu$ , as a function of compression is shown for one network in Fig.S2. The Poisson's ratio is still trainable to a value of nearly 0 even at a lower temperature.

Temperature couples with training duration to modify the relaxation time of the trained behavior. In the experiments described above networks were trained both for less time overall and at lower temperatures than those described in the reported results. The Poisson's ratio is measured immediately after training and a sharp decrease is observed. However, within 24hrs we find that the Poisson's ratio has relaxed back to nearly its initial value. For the experiments reported in this paper using the described training procedure for longer duration and higher temperature we find that arrays can sustain a negative Poisson's ratio value at least 23 days later as shown in Fig.S3. Pashine *et. al.* describe a similar relation between training duration and relaxation time for EVA foam arrays[1].

**Instrumentation**

**Differential Scanning Calorimetry (DSC)-** DSC measurements were conducted using a TA Instruments Discovery 2500 differential scanning calorimeter. Samples were placed in aluminum hermetic pans from TA Instruments, and the experiments followed these steps: an initial heating cycle (22 °C to 200 °C), a cooling cycle (200 °C to -90 °C), a second heating cycle (-90 °C to 200 °C), and a final cooling cycle (200 °C to -90 °C). Both heating and cooling cycles were performed at a rate of 10 °C/min. The curves from the second heating cycle are presented in this paper.

## Synthesis schemes

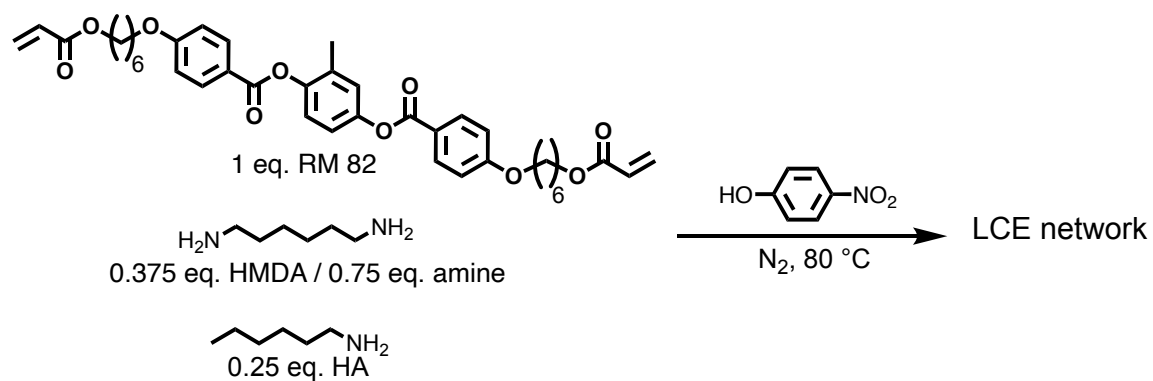

Liquid crystal elastomer (LCE) synthesis scheme

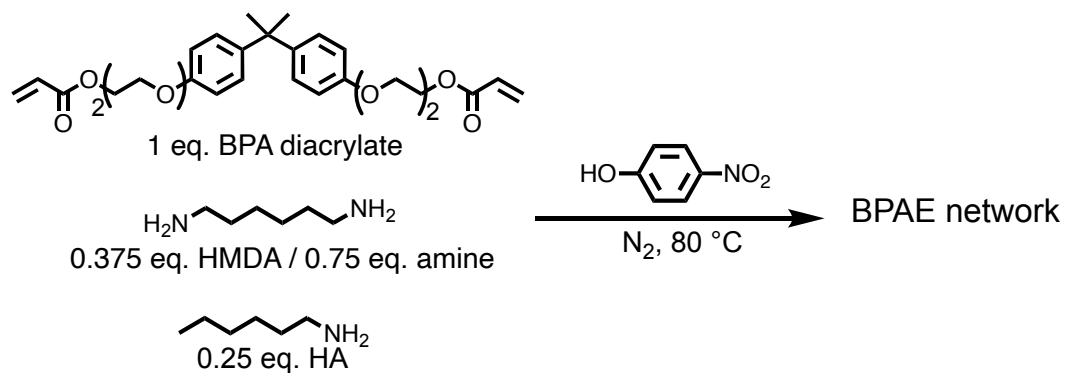

Bisphenol-A elastomer (BPAE) synthesis scheme

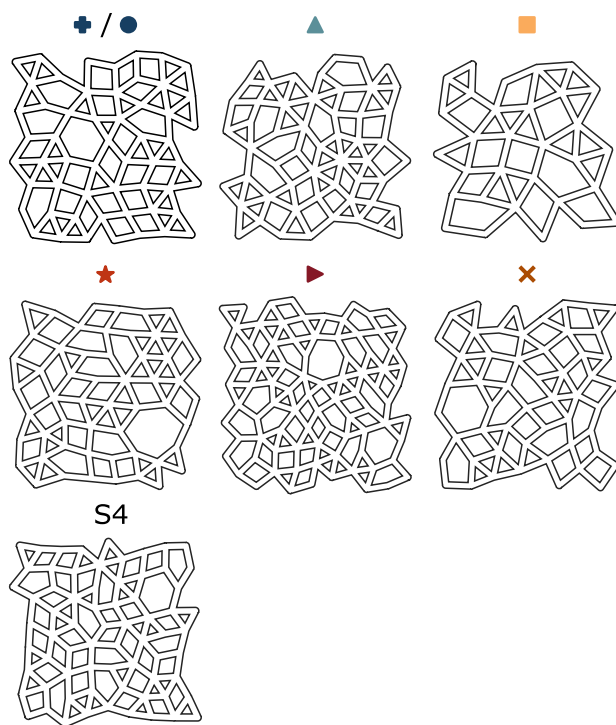

**Fig. S1.** The six disordered array geometries shown in Fig.1 are shown here with the symbol above corresponding to the matching data in that figure. A seventh geometry used for experiments in Fig.S2 is labeled S1.

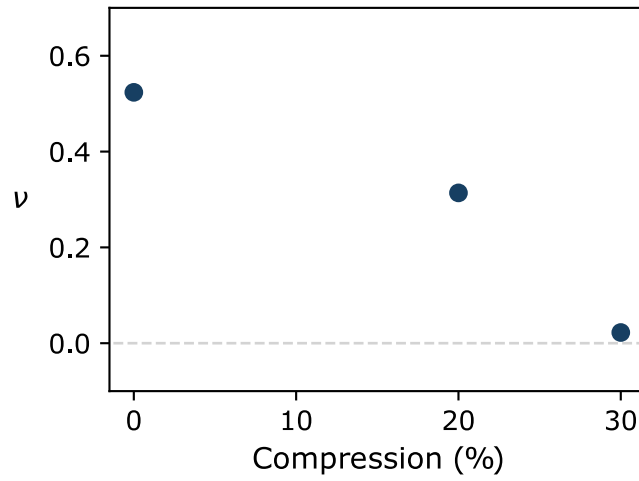

**Fig. S2.** The Poisson's ratio,  $\nu$ , as a function of compression for a network training at 50C for less than 24hrs as a function of training compression.

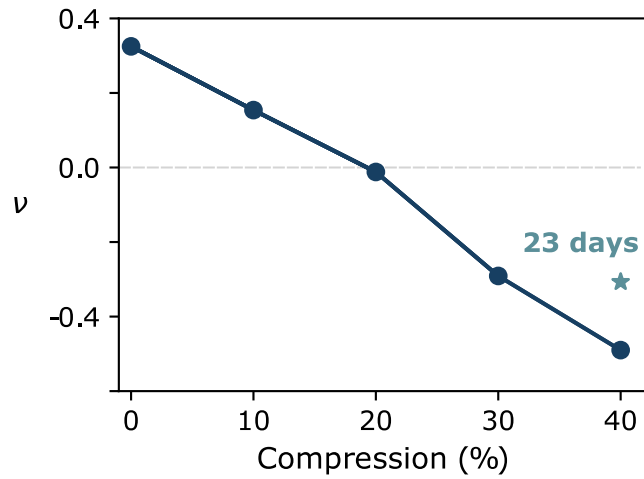

**Fig. S3.** The Poisson's ratio,  $\nu$ , as a function of compression for one network as reported in the manuscript is shown. The array is remeasured after a rest period of 23 days shown by the star. Some relaxation is observed, but the array sustains auxetic behavior over a duration much longer than its initial training time.

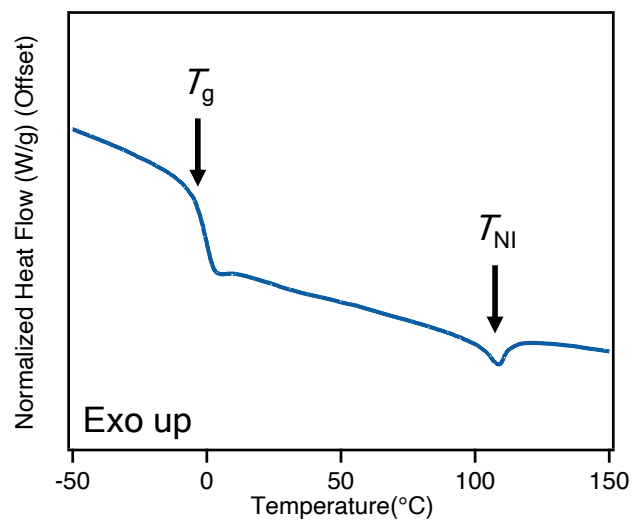

**Fig. S4.** DSC of LCE showing the glass transition temperature ( $T_g$ ) and the nematic to isotropic transition temperature ( $T_{NI}$ ).



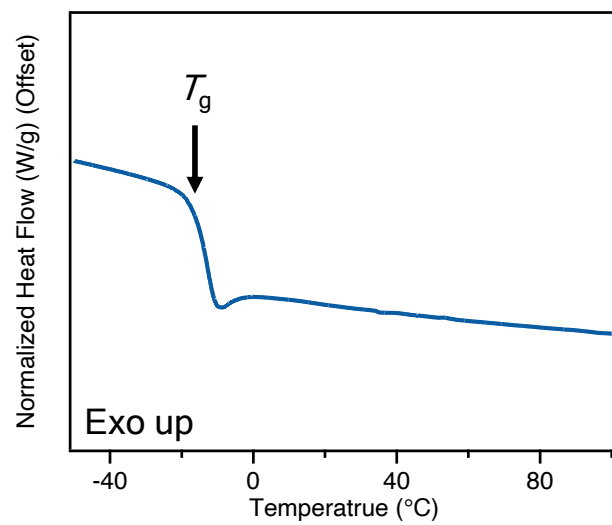

**Fig. S5.** DSC of BPAE showing the glass transition temperature ( $T_g$ ).

## SI References

1. Pashine, Nidhi, et al. "Directed aging, memory, and nature's greed." *Science advances* 5.12 (2019): eaax4215.
